# Supplementary material for: Noise2Void - Learning Denoising from Single Noisy Images
Source: arXiv:1811.10980 ancillary file (2019-04-05)
Supplement: Supplementary file 1 [file supp_small.pdf]

# Noise2Void - Learning Denoising from Single Noisy Images Supplementary Note

Alexander Krull[1,2], Tim-Oliver Buchholz[2], Florian Jug

[1] krull@mpi-cbg.de

[2] Authors contributed equally

MPI-CBG/PKS (CSBD), Dresden, Germany

This supplementary note provides additional information on NOISE2VOID and on the experiments we conducted. We will first discuss details on our training, validation and and data preparation procedure (Section 1) and then continue to provide the size of our networks' receptive fields (Section 2). Finally, we will provide additional results achieved by multiple variations of our method (Section 3).

In Supplementary Figures 1, 2, 3, and 4 we will show additional qualitative results.

# 1 Training, Validation and Data Preparation

We train all networks for 200 cycles, with each cycle consisting of 400 gradient steps. During the training of all networks we perform on-the-fly random sub-patch extraction (with a size of $64 \times 64$) from our previously prepared training data.

The validation loss, which is used by the CARE learning rate scheduler, is calculated like the training loss for traditional training, N2N, and N2V respectively. Using the ground truth for traditional training, and a second noisy image for N2N. For N2V, we calculate the validation loss using randomly selected masked pixels, like it is done for the training loss.

We will now go on to describe the training data preparation of the individual datasets and provide additional details.

## 1.1 BSD68 [2]

As in [4], we train our network using the 400 gray scale images with $180 \times 180$ pixels. We add zero centered independent Gaussian noise ($\sigma = 25$) to all patches. Then we randomly select 1% of all patches to serve as validation dataset. Finally, we augment our data by adding all rotated (multiples of $90°$) and mirrored versions. During training with N2V, we use the *Uniform Pixel Selection* UPS masking method with a $5 \times 5$ pixel window (see Section 3.1).

## 1.2 Simulated Microscopy

In the simulation of our microscopy data, we start out with three independently generated 3D phantom image stacks (size: $256 \times 256 \times 256$) that describe the fluorophore distribution in our sample. We use two of the phantoms to generate training data and one to generate test data. We start the microscope simulation by normalizing the phantoms to the range $[0, 1]$. We than add a constant value of 0.2 to simulate background illumination and multiply the phantoms by a factor $\lambda$ to account for the exposure. Subsequently we simulate shot noise. Every pixel value is generated by drawing from a Poisson distribution using the shifted and scaled phantom as the expected value of the pixel. Finally, we add pixel-wise independent zero-mean Gaussian noise with a standard deviation of $\sigma = 1$ to simulate readout noise in the sensor. According to the above scheme, we generate low- and high-exposure-images, using $\lambda = 20$ and $\lambda = 10000$ respectively. A second low-exposure-image ($\lambda = 20$) is generated for N2N training. The high-exposure-images serve as ground truth for the traditional training and are used to calculate the PSNR during testing. With respect to the latter, we account for different exposure rates by scaling our network output with the corresponding factor. Since N2V is currently only implemented in 2D, we view each of the generated 3D image stacks as collection of 2D images and process them independently. We use 10% of out training images as validation dataset. During training with N2V, we use the *Gaussian Pixel Selection* (GPS) masking method (see Section 3.1).

## 1.3 Fluo-C2DL-MSC (CTC-MSC) [3]

We train our network using the two training movies provided in the *cell tracking challenge*[1]. We use **only** the image data without any additional annotations like ground truth segmentations. This is the same data we use for testing as well. We iterate over all frames of both movies and randomly extract patches of $80 \times 80$ pixels. To reduce the amount of patches showing only background we calculate the standard deviation of the intensities of each patch. We exclude all patches with standard deviation below 1250. For each frame we continue to sample until we find 256 patches that pass this test. We use one of these patches from every frame in our validation set. We augment our data by adding all rotated (multiples of $90°$) and mirrored versions. During training with N2V, we use the UPS masking method with a $5 \times 5$ pixel window (see Section 3.1).

[1] http://celltrackingchallenge.net/

### 1.4 Fluo-N2DH-GOWT1 (CTC-N2DH) [3]

The Fluo-N2DH-GOWT1 training dataset also consists of two movies. Again we use **only** the image data without any additional annotations like ground truth segmentations. This is again the same data we use for testing as well. The data preparation is done as for the CTC-MSC dataset. However, here we exclude all patches with standard deviation below 5. During training with N2V, we use the UPS masking method with a $5 \times 5$ pixel window (see Section 3.1).

### 1.5 Cryo-TEM [1]

We use a single $7676 \times 7420$ pixel cryo-TEM image as source for our training data and extract 435 overlapping patches of size $512 \times 512$. The same image is later used for testing. We randomly select $10\%$ of the patches and use them as validation dataset. Here, we do not use data augmentation in the form of flipping or rotating. During training with N2V, we use the UPS masking method with a $5 \times 5$ pixel window (see Section 3.1).

## 2 Receptive Fields of our Networks

We used the CARE framework to calculate the size of our networks' receptive fields: A CARE network with kernel size of $3 \times 3$ and depth 2 has a receptive field of $22 \times 22$ pixels. A network with kernel size of $5 \times 5$ has a receptive field of size $40 \times 40$.

## 3 Variations of N2V and Parameters

We used the BSD68 dataset to test different parameter settings and to try different variants of our masking scheme. The results can be found in Supplementary Table 1.

### 3.1 Masking Methods

We tried the following variants of our masking scheme: **Uniform Pixel Selection (UPS)** replaces the value of the selected pixel $i$ with a randomly selected pixel value from a square window around $i$. This includes the pixel itself. In Supplementary Table 1 we write the size of the window in parenthesis.
**Gaussian (G)** masking changes the value of the selected pixel $i$ by adding random Gaussian noise. In Supplementary Table 1 we provide the standard deviation of the noise in parenthesis.
The **Gaussian Fitting (GF)** method looks at a local square neighborhood of the pixel $i$ and fits a 1D Gaussian distribution to the pixel values by calculating mean and standard deviation. The pixel $i$ is included in this calculation. The pixel value is masked by drawing from the fitted Gaussian distribution. In Supplementary Table 1 we write the size of the neighborhood in parenthesis.
The **Gaussian Pixel Selection (GPS)** replaces the value of the selected pixel $i$ with a randomly selected pixel that is found by drawing from a 2D isotropic Gaussian distribution centered at pixel $i$. The pixel $i$ itself is excluded from this draw. That is, if the pixel $i$ is selected by the Gaussian draw, we redraw until another pixel has been selected. We use a Gaussian distribution with a standard deviation of $\sigma = 4$.

Masking Types

| Masking | Kernel | Loss | Features | PSNR |
|---|---|---|---|---|
| UPS (3×3) | 3×3 | MSE | 96 | 26.98 |
| UPS (5×5) | 3×3 | MSE | 96 | 27.71 |
| UPS (7×7) | 3×3 | MSE | 96 | 27.26 |
| UPS (50×50) | 3×3 | MSE | 96 | 27.42 |
| GF (3×3) | 3×3 | MSE | 96 | 27.51 |
| GF (5×5) | 3×3 | MSE | 96 | 27.31 |
| GF (7×7) | 3×3 | MSE | 96 | 27.47 |
| GF (50×50) | 3×3 | MSE | 96 | 27.35 |
| G (5) | 3×3 | MSE | 96 | 27.24 |
| G (10) | 3×3 | MSE | 96 | 26.52 |
| GPS | 3×3 | MSE | 96 | 27.31 |

Other Parameters

| Masking | Kernel | Loss | Features | PSNR |
|---|---|---|---|---|
| UPS (5×5) | 5×5 | MSE | 96 | 27.60 |
| UPS (5×5) | 3×3 | MAE | 96 | 27.58 |
| UPS (5×5) | 5×5 | MAE | 96 | 26.99 |
| UPS (5×5) | 3×3 | MAE | 32 | 27.33 |
| UPS (5×5) | 5×5 | MAE | 32 | 27.36 |

Table 1: Results achieved with various masking methods and different parameter settings on the BSD68 dataset.

### 3.2 Other Parameters

In addition to the masking method, we also experimented with other parameters. In particular, we tried using the mean absolute error (MAE) as our loss function instead of the mean square error (MSE). We also varied the number of feature channels used in the first layer, denoted as *Features* in Supplementary Table 1, and the size of the convolutional kernels used in the network, denoted as *Kernel*.

## References


[1] T.-O. Buchholz, M. Jordan, G. Pigino, and F. Jug. Cryo-care: Content-aware image restoration for cryo-transmission electron microscopy data. *arXiv preprint arXiv:1810.05420*, 2018. 2

[2] S. Roth and M. J. Black. Fields of experts. *International Journal of Computer Vision*, 82(2):205, 2009. 1

[3] V. Ulman, M. Maška, K. E. Magnusson, O. Ronneberger, C. Haubold, N. Harder, P. Matula, P. Matula, D. Svoboda, M. Radojevic, et al. An objective comparison of cell-tracking algorithms. *Nature methods*, 14(12):1141, 2017. 1

[4] K. Zhang, W. Zuo, Y. Chen, D. Meng, and L. Zhang. Beyond a gaussian denoiser: Residual learning of deep cnn for image denoising. *IEEE Transactions on Image Processing*, 26(7):3142–3155, 2017. 1

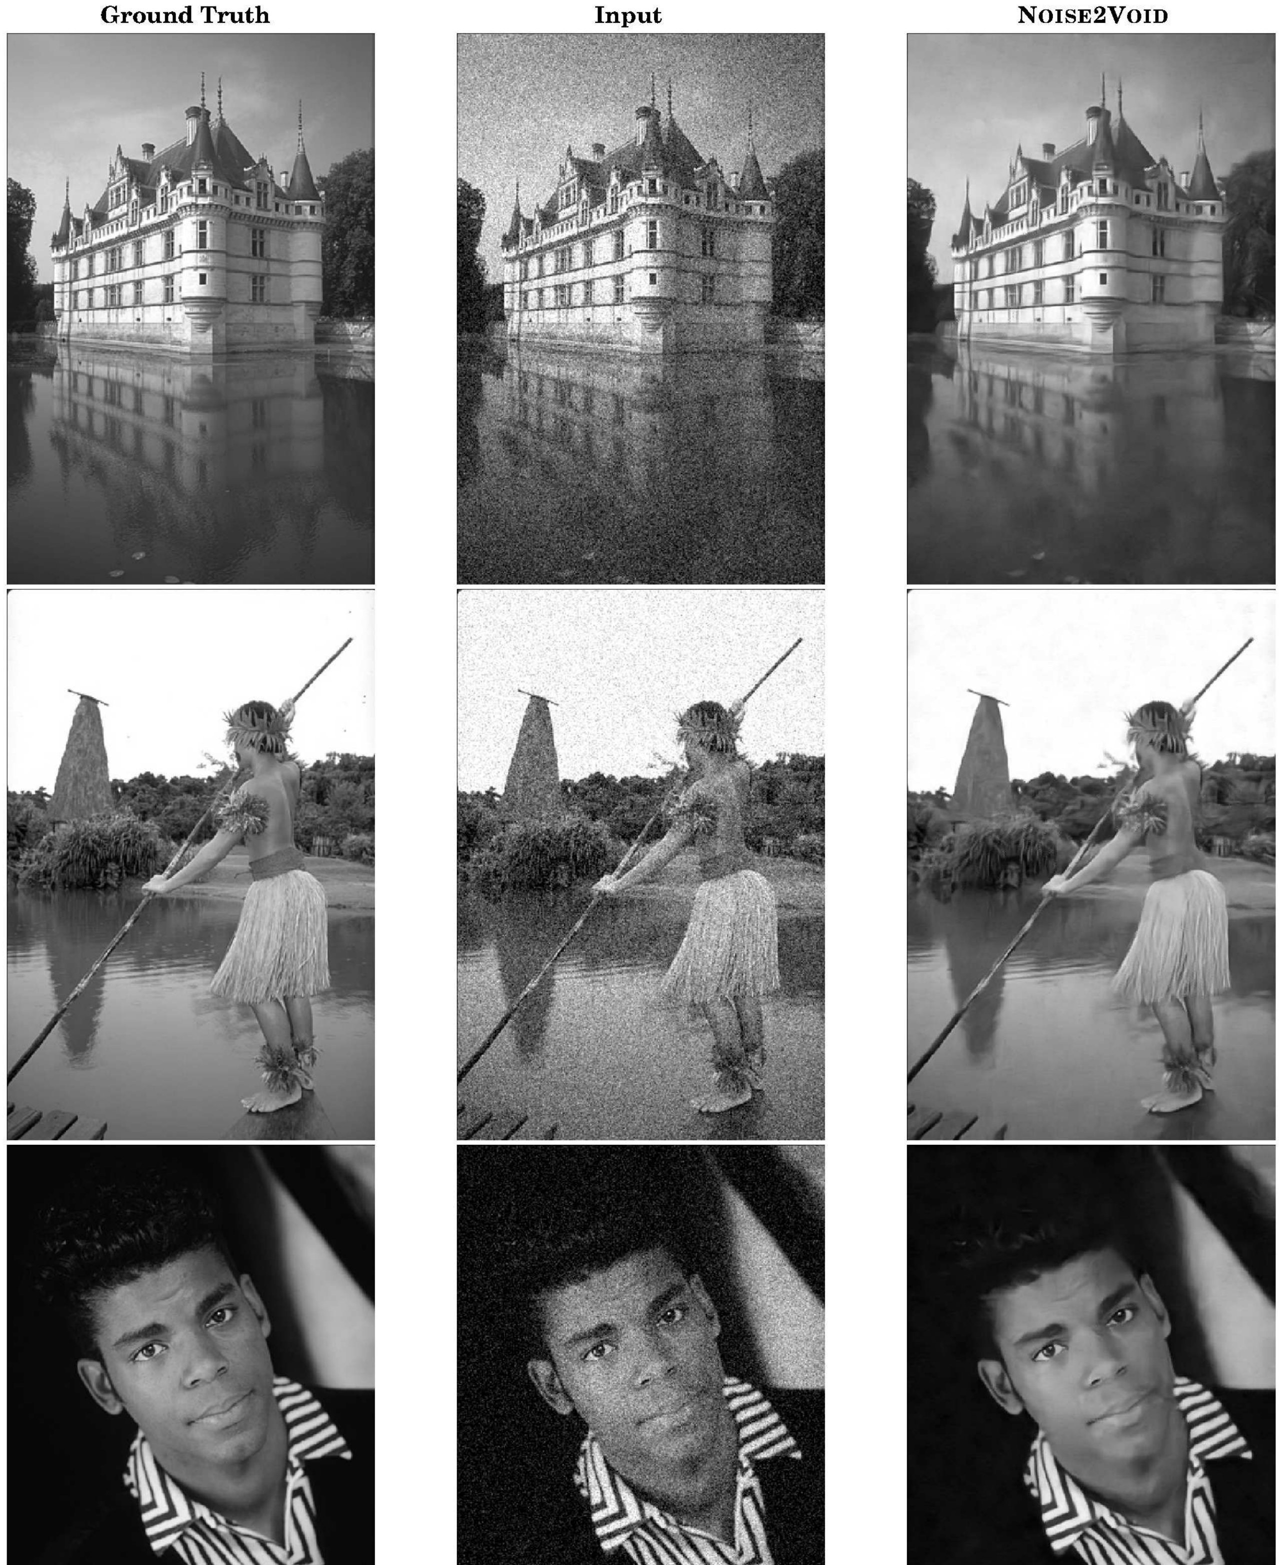


Figure 1: Qualitative NOISE2VOID results on the BSD68 dataset.

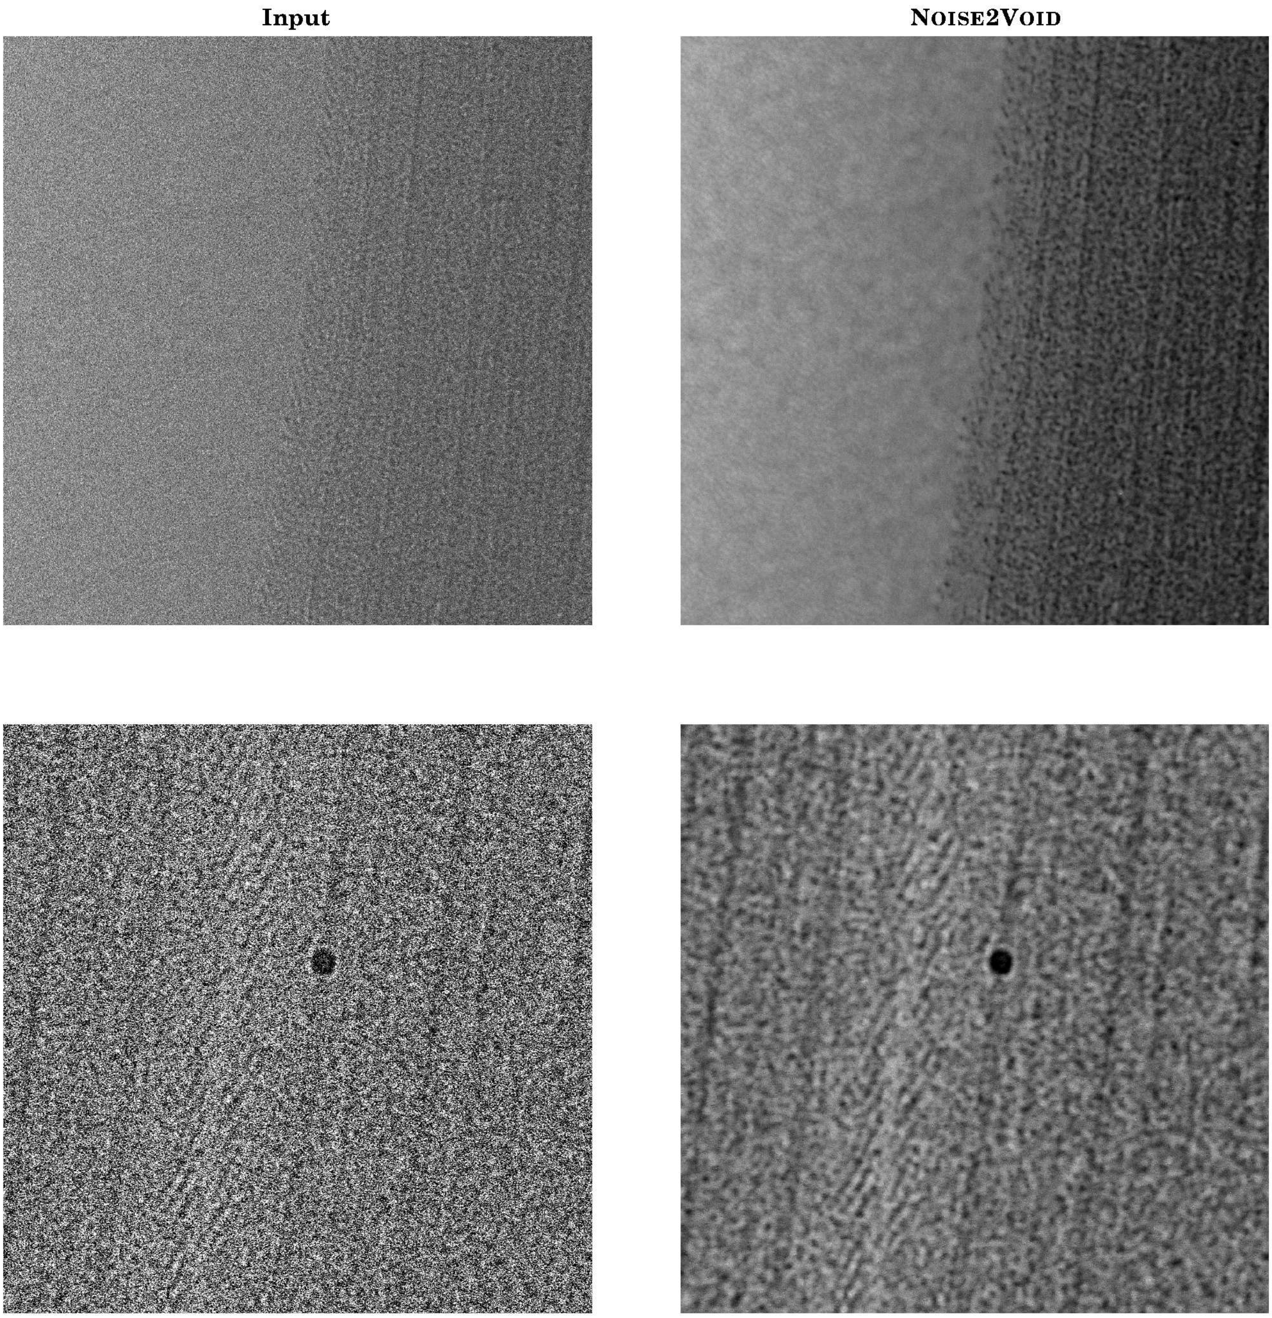


Figure 2: Qualitative NOISE2VOID results from the cryo-TEM dataset.

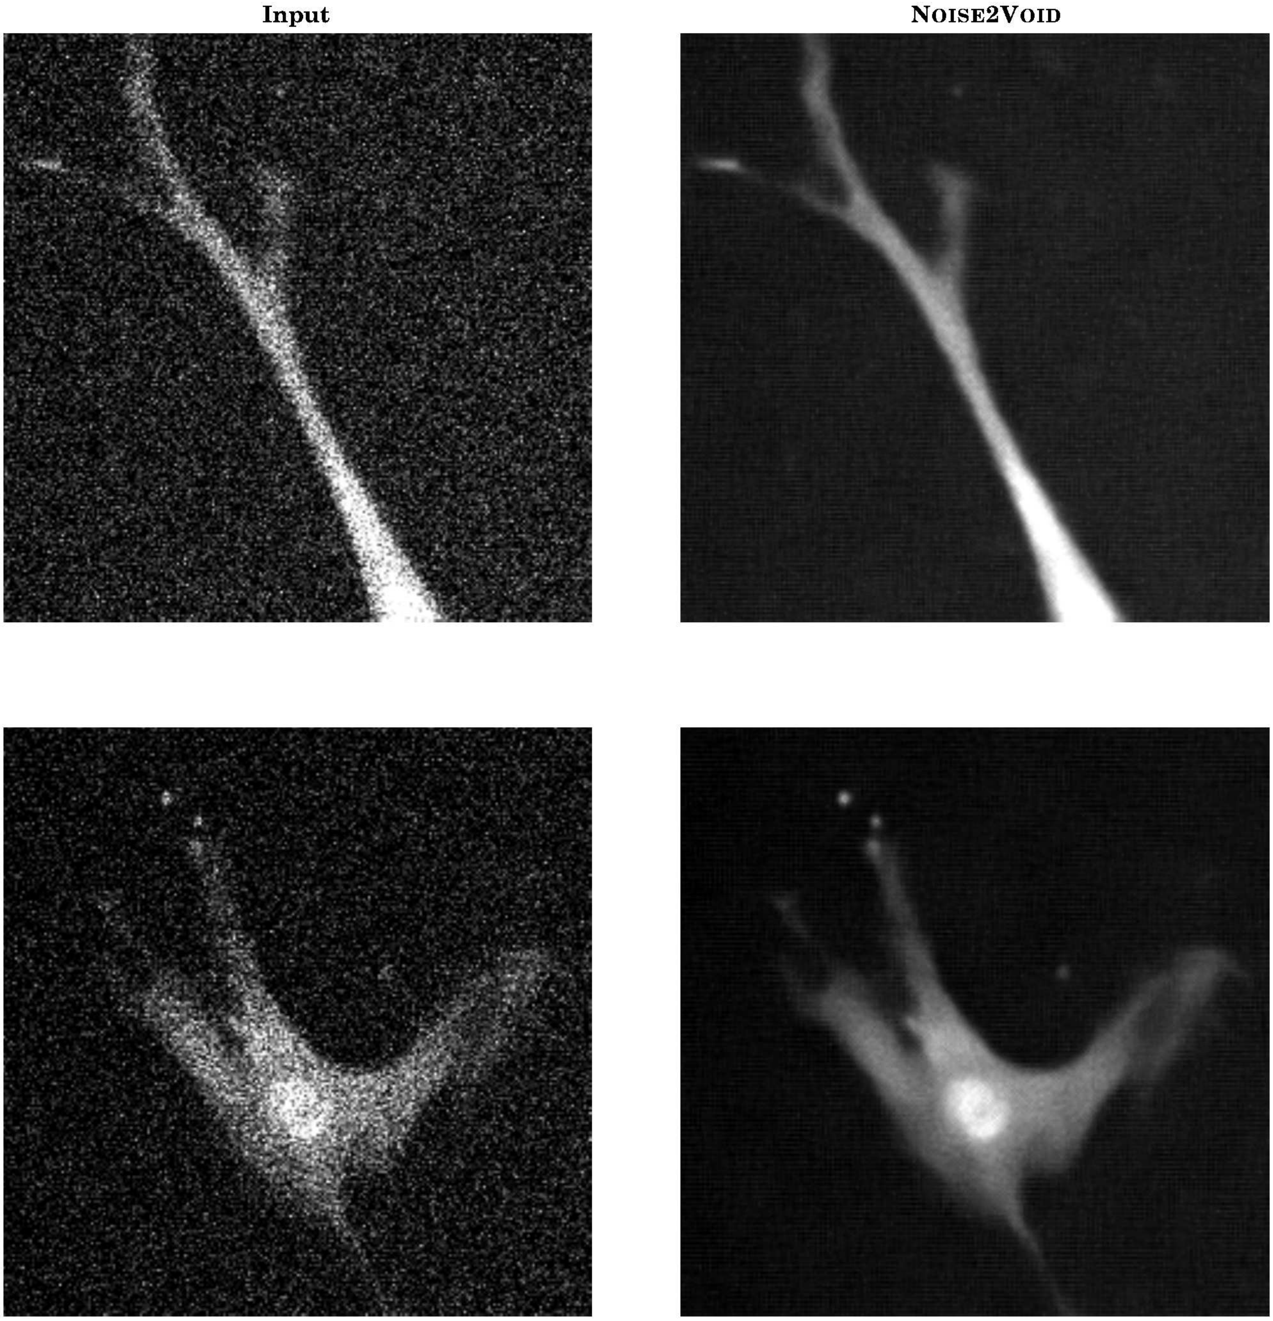


Figure 3: Qualitative NOISE2VOID results from the CTC-MSC Dataset.

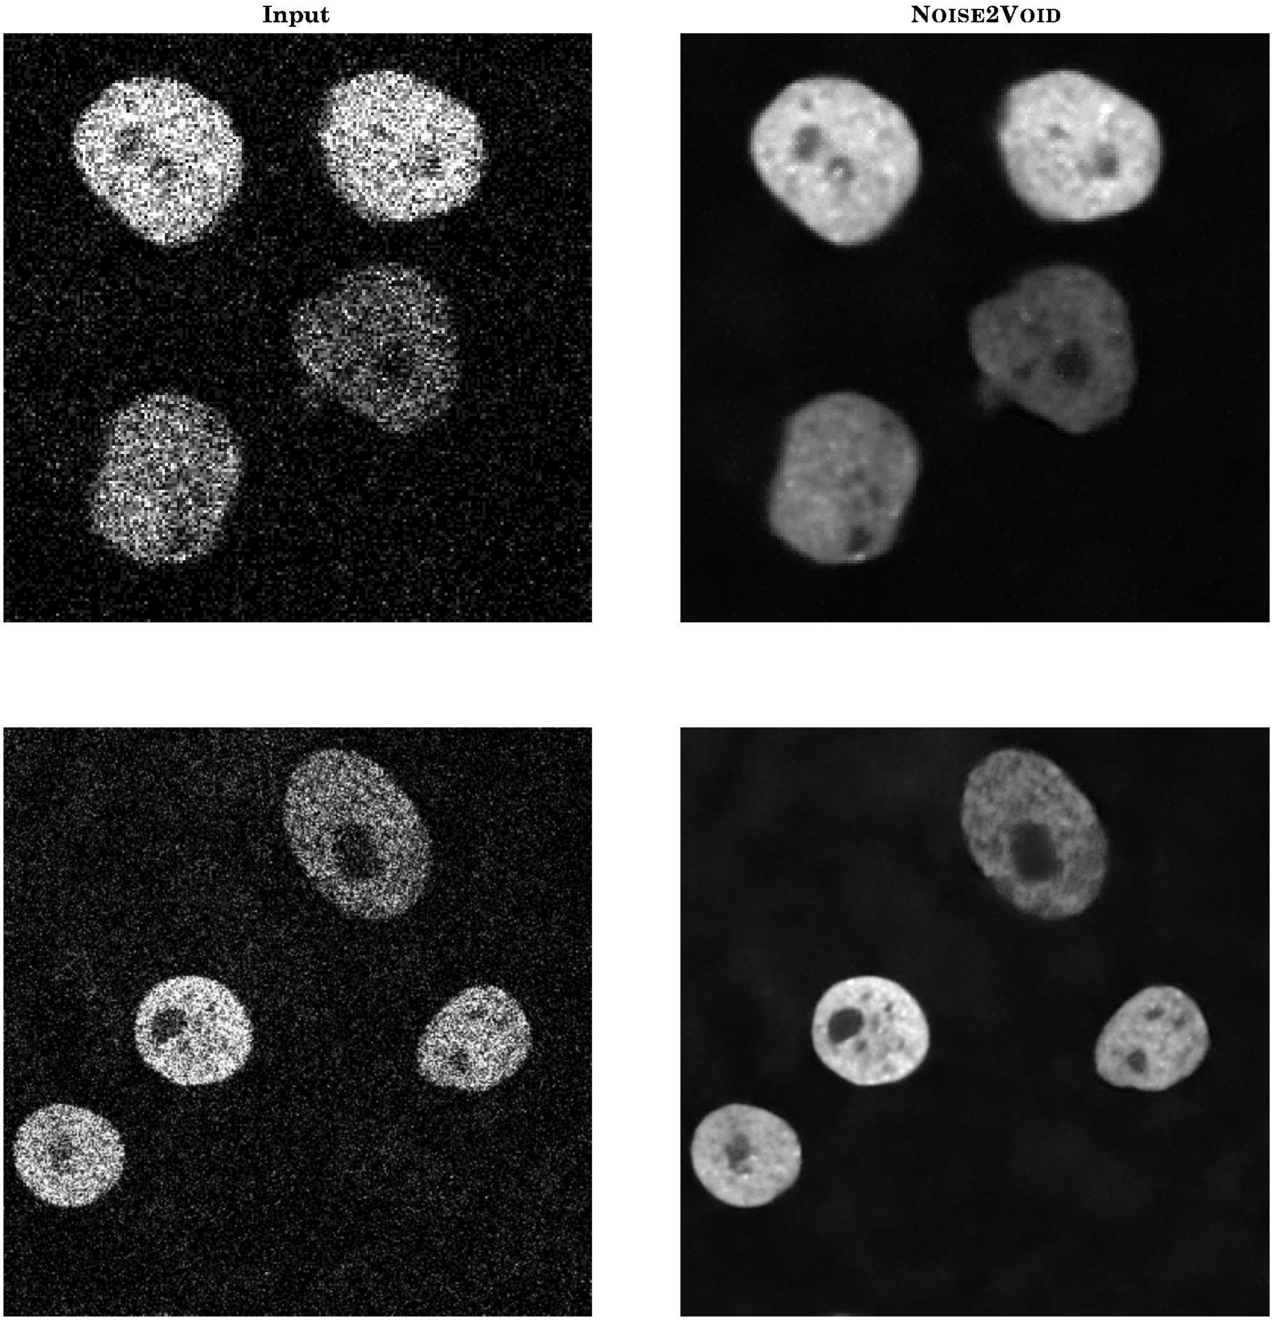


Figure 4: Qualitative Noise2Void results from the CTC-N2DH dataset.
